# Supplementary material for: Redundancies in Dependently Typed Lambda Calculi and Their Relevance to Proof Search
Source: arXiv:1007.0779 source file (2010-07-05)
Supplement: Supplementary file 1 [file appendix.tex]

\appendix

\section{Proofs of Theorems} \label{appendix:proofs}

\subsection{Correctness of the simplified encoding\\
  (Theorem~\ref{theorem:simplified-translation-correctness})}

\subsubsection{Completeness}

We use induction on the derivation
of $\lfprove{\Gamma}{\oftype{M}{A}}$ to build one for
$\iprove{\enc{\Gamma}}{\enc{\oftype{M}{A}}}$.
We proceed by case analysis on the canonical type $A$.

\smallskip
\noindent If $A$ is of the form $\typedpi{x}{B}{A'}$ then $M$ must be
of the form $\typedlambda{x}{B}{M'}$ and the LF derivation
must end with an \absobj\ rule, \ie, a rule of the form
\[
   \AxiomC{$\lfprove{\Gamma}{\oftype{A'}{\type}} \quad
     \lfprove{\Gamma,\oftype{x}{B}}{\oftype{M}'{A'}}$}
   \RightLabel{\absobj}
   \UnaryInfC{$\lfprove{\Gamma}{
      \oftype{(\typedlambda{x}{B}{M'})}{(\typedpi{x}{B}{A'})}}$}
   \DisplayProof
\]
The induction hypothesis gives us a derivation for
\begin{tabbing}
\qquad\=\kill
\>$\iprove{\enc{\Gamma, \oftype{x}{B}}}{\enc{\oftype{M'}{A'}}}$.
\end{tabbing}
By applying the rules \allGoal\ and \impGoal\ to this, we get a
derivation for 
$\iprove{\enc{\Gamma}}{
    \forall x.~ \enc{\oftype{x}{B}} \supset \enc{\oftype{M'}{A'}}}$.
The righthand side of this sequent is the expected goal:
\begin{tabbing}
\qquad\=\qquad\qquad\=\kill
\>$\enc{\oftype{(\typedlambda{x}{B}{M'})}{(\typedpi{x}{B}{A'})}} =$\\
\>\>$\forall x.~ \enc{\oftype{x}{B}} \supset
(\enc{A'} \ (\encTerm{\typedlambda{x}{B}{M'}} \ x))$,
\end{tabbing}
and $\encTerm{M'} = (\encTerm{\typedlambda{x}{B}{M'}}\app x)$ by virtue of
$\eta$-conversion. 

\medskip
\noindent If $A$ is a base type then $M$ must be of the form
$x\app N_1 \app \ldots \app N_n$ and the canonical LF derivation must
end with a chain of \appobj\ rules following a \varobj\ rule that
reveals that 
\begin{tabbing}
\qquad\=\kill
\>$\oftype{x}{\typedpi{y_1}{B_1}{\ldots\typedpi{y_n}{B_n}{A'}}}\in\Gamma$.
\end{tabbing}
Moreover, $A$ must be $A'\subst{{N_1/y_1,\ldots,N_n/y_n}}$ and, from looking at the right
upper premise of the \appobj\ rules, there must be shorter derivations
of 
\begin{tabbing}
\qquad\=\kill
\>$\lfprove{\Gamma}{\oftype{N_i}{B_i\subst{N_1/x_1,\ldots,N_{i-1}/x_{i-1}}}}$
\end{tabbing}
for $1 \leq i \leq n$. By the induction hypothesis we obtain
derivations ${\cal D}_i$ of $\iprove{\enc{\Gamma}}{ 
   \enc{\oftype{N_i}{B_i\subst{N_1/x_1, \ldots, N_{i-1}/x_{i-1}}}}}$.
Further, $\enc{\Gamma}$ must contain 
\begin{tabbing}
\qquad\=\qquad\=\kill 
\>$\forall y_1.~ (\enc{B_1} \app y_1) \supset \ldots \supset$\\
\>\>$\forall y_n.~ (\enc{B_n} \app y_n) \supset
     hastype \app (x \app y_1 \app \ldots\app y_n) \app \encTerm{A'}$,
\end{tabbing}
\ie, the encoding of
     $\oftype{x}{\typedpi{y_1}{B_1}{\ldots\typedpi{y_n}{B_n}{A'}}}$.
By applying \bcGoal\ on that clause,
choosing $\encTerm{N_i}$ for $y_i$
and using the derivations ${\cal D}_i$,
we obtain a derivation of
\begin{tabbing}
\qquad\=$\iprove{\enc{\Gamma}}{hastype \app}$\=\kill
\>$\iprove{\enc{\Gamma}}{hastype \app
(x \app \encTerm{N_1}\app\ldots\app \encTerm{N_n})$\\
\>\>$(\encTerm{A'}\subst{\encTerm{N_1}/y_1,\ldots
                           \encTerm{N_n}/y_n})}$.
\end{tabbing}
The right side of this sequent is precisely
\begin{tabbing}
\qquad\=\kill
\>$\enc{\oftype{(x \app N_1 \app\ldots\app
N_n)}{A'\subst{N_1/y_1,\ldots,N_n/y_n}}}$.  
\end{tabbing}

\subsubsection{Soundness}

We prove the soundness direction by induction on the derivation of
$\iprove{\enc{\Gamma}}{(\enc{A}\app M)}$: assuming that
$\lfprove{\Gamma}{\oftype{A}{\type}}$ has a derivation,
we establish that $M = \encTerm{M'}$ for some canonical object $M'$
and we build a derivation of $\lfprove{\Gamma}{\oftype{M'}{A}}$.
A case analysis on the structure of the canonical type $A$
will guide us.

\smallskip
\noindent If $A$ is of the form $\typedpi{x}{B}{A'}$ then the structure of
$\enc{A}$ forces the \hhf\ derivation to conclude as follows:
\[
  \AxiomC{$
    \iprove{\enc{\Gamma,\oftype{x}{B}}}{(\enc{A'}\app (M\app x))}
  $}
  \RightLabel{\allGoal, \impGoal}
  \doubleLine
  \UnaryInfC{$\iprove{\enc{\Gamma}}{
     \forall x.~ (\enc{B}\app x) \supset (\enc{A'}\app (M\app x))}$}
  \DisplayProof
\]
Since $A$ is a valid $\type$ under $\Gamma$, $B$ must also be,
and $A'$ must be valid under $(\Gamma,\oftype{x}{B})$.
We can thus apply the inductive hypothesis,
and we obtain that $M\app x = \encTerm{M'}$ 
and that $\lfprove{\Gamma,\oftype{x}{B}}{\oftype{M'}{A'}}$ is
derivable for some canonical object $M'$.
Since $x$ does not occur free in $M$, we conclude that
\begin{tabbing}
\qquad\=\kill
\>$M = (\lambda x. \encTerm{M'}) = \encTerm{\typedlambda{x}{B}{M'}}$,
\end{tabbing}
and we derive
$\lfprove{\Gamma}{\oftype{(\typedlambda{x}{B}{M'})}{(\typedpi{x}{B}{A'})}}$
using the \absobj\ rule and our derivation of
$\lfprove{\Gamma}{\oftype{B}{\type}}$.

\medskip
\noindent
Otherwise, $A$ is a base type, and the derivation we are considering
is that of $\iprove{\enc{\Gamma}}{hastype\app
M\app \encTerm{A}}$. This derivation must end in a \bcGoal\ rule that
uses some clause in $\enc{\Gamma}$ of the form
\begin{tabbing}
\qquad\=\qquad\=\kill
\>$\forall y_1.~ (\enc{B_1}\app y_1) \supset \ldots \supset$\\
\>\>$\forall y_n.~ (\enc{B_n} \app y_n) \supset
     hastype \app (x \app y_1 \app\ldots\app y_n) \app \encTerm{A'}$;
\end{tabbing}
note that the variables $y_1,\ldots,y_{i-1}$ can appear in $\enc{B_i}$
here. 
Thus, for some \hhf\ terms $N_1,\ldots,N_n$, 
\begin{tabbing}
\qquad\=\kill
\>$\encTerm{A} = \encTerm{A'}\subst{N_1/y_1,\ldots,N_n/y_n}$,
\end{tabbing}
$M = (x\app N_1\app \ldots\app N_n)$, and, for each $i$ such that
$1 \leq i \leq n$, there is a shorter derivation of
\begin{tabbing}
\qquad\=\kill
\>$\iprove{\enc{\Gamma}}{(\enc{B_i} \
y_i)\subst{N_1/y_1,\ldots,N_i/y_i}}$,
\end{tabbing}
\ie, of $\iprove{\enc{\Gamma}}{
           (\enc{B_i}\subst{N_1/y_1,\ldots,N_{i-1}/y_{i-1}}\app N_i})$.
Further, we know that
$\oftype{x}{\typedpi{y_1}{B_1}{\ldots\typedpi{y_n}{B_n}A'}}\in\Gamma$ for 
some $x$. We now claim that, for $1 \leq i\leq n$,
$N_i = \encTerm{N'_i}$ for some canonical LF object $N'_i$ and
that $\lfprove{\Gamma}{\oftype{N'_i}{B_i \subst{N'_1/y_1\ldots
N'_{i-1}/y_{i-1}}}}$ has a derivation. If this claim is true, then,
we can use the \varobj\ rule to derive
$\lfprove{\Gamma}{\oftype{x}{\typedpi{y_1}{B_1}{\ldots\typedpi{y_n}{B_n}A'}}}$
and follow this by a sequence of \appobj\ rule applications to prove
$\lfprove{\Gamma}{\oftype{(x \app N'_1\app \ldots\app N'_n)}{
                          A'\subst{N'_1/y_1 \ldots N'_n/y_n}}}$. 
Now, evidently $M = \encTerm{x\app N'_1\app\ldots\app N'_n}$ and,
since substitution permutes with encoding, $A = A'\subst{N'_1/y_1,\ldots,N'_n/y_n}$. Thus, the desired result would
be proven. 

It only remains, then, to establish the claim. We actually strengthen
it to include also the assertion that, for $1 \leq i \leq
n$, $\lfprove{\Gamma}{\oftype{B_i\subst{N'_1/y_1 \ldots
N'_{i-1}/y_{i-1}}}{\type}}$ has a derivation. To prove it, we use an
inner induction on 
$i$. Since $\Gamma$ is a well-formed context, and
$\oftype{x}{\typedpi{y_1}{B_1}{\ldots\typedpi{y_n}{B_n}A'} \in \Gamma$,
there must be a derivation of 
\[\lfprove{\Gamma,\oftype{x_1}{B_1},\ldots,\oftype{x_{i-1}}{B_{i-1}}}
            {\oftype{B_i}{\type}}\] 
for $1 \leq i \leq n$. Using Proposition~\ref{prop:lf-substitution}
and the induction hypothesis we see that there must be a
derivation of 
\[\lfprove{\Gamma}{\oftype{B_i\subst{N'_1/y_1 \ldots 
      N'_{i-1}/y_{i-1}}}{\type}}.\]
Noting that \[\enc{B_i}\subst{N_1/y_1,\ldots,N_{i-1}/y_{i-1}}}
      = \enc{B_i\subst{N_1/y_1,\ldots,N_{i-1}/y_{i-1}}},\] 
the outer induction hypothesis and the shorter derivation
      of $\iprove{\enc{\Gamma}}{
           (\enc{B_i}\subst{N_1/y_1,\ldots,N_{i-1}/y_{i-1}}\app N_i})$
          allows us to conclude that $N_i = \encTerm{N'_i}$ for some
          canonical LF term $N'_i$ and that there is a derivation
           of \[\lfprove{\Gamma}{\oftype{N'_i}{B_i \subst{N'_1/y_1\ldots
N'_{i-1}/y_{i-1}}}},\] thus verifying the claim. 

\subsection{Completeness of the optimized encoding
  (Theorem~\ref{theorem:extended-translation-equivalence})}
                                   
If $\iprove{\enc{\Gamma}}{\enc{A} M}$ has a derivation, then
$\iprove{\encExtP{\Gamma}{}}{\encExtN{A} M}$ has a derivation as well.
Note that for this direction of the proof we are simply dropping
information (subderivations) and so we do not
rely on $\Gamma$ being a valid specification or
$A$ being a valid type.
We proceed by induction on the structure of the derivation of
$\iprove{\enc{\Gamma}}{\enc{A} M}$, followed by case analysis on $A$.

\smallskip
\noindent 
If $A$ is of the form $\typedpi{x}{B}{A'}$ our derivation ends as follows:
\[
    \AxiomC{$\iprove{\enc{\Gamma, \oftype{x}{B}}}{\enc{A'} \ (M \app x)}$}
    \RightLabel{\allGoal, \impGoal}
    \doubleLine
    \UnaryInfC{$\iprove{\enc{\Gamma}}
                       {\enc{\typedpi{x}{B}{A'}} \ M}$}
\DisplayProof
\]
By the inductive hypothesis
$\iprove{\encExtP{\Gamma, \oftype{x}{B}}{}}{\encExtN{A'} \ (M \app x)}$ has a
derivation, and by applying \allGoal\ and \impGoal\ to this derivation we can
construct a derivation of
\[ \iprove{\encExtP{\Gamma}{}}
        {\encExtN{\typedpi{x}{B}{A'}} \ M} \]

\smallskip
\noindent
Otherwise, $A$ is a base type and our derivation proceeds by backchaining
on some $(\oftype{y}{\typedpis{x}{B}{A'}})\in\Gamma$,
with $\encTerm{A}=\encTerm{A'}\subst{t_1/x_1\ldots t_n/x_n}$:
\[
    \AxiomC{$\iprove{\enc{\Gamma}}{F_1}
             \quad \ldots \quad
             \iprove{\enc{\Gamma}}{F_n}$}
    \RightLabel{\bcGoal}
    \UnaryInfC{$\iprove{\enc{\Gamma}}
                       {\enc{A} \ (y \vec{t})}$}
\DisplayProof
\]
Here, $F_i = (\enc{B_i} \ x_i)\subst{t_1/x_1\ldots t_n/x_n}$.
As in the completeness proof of the simplified encoding,
we obtain by an inner induction that each $t_i$ is of the form
$\encTerm{t'_i}$ and thus that
$F_i = \enc{B_i\subst{t'_1/x_1\ldots t'_n/x_n}}(t_i)$.
We shall build the derivation of
$\iprove{\encExtP{\Gamma}{}}{\encExtN{A}(y \vec{t})}$
by using \bcGoal\ on the optimized encoding of
$(\oftype{y}{\typedpis{x}{B}{A'}})\in\Gamma$,
by choosing $\vec{t}$ for $\vec{x}$.
The resulting premises are either
\[ \iprove{\encExtP{\Gamma}{}}{
   \encExtN{B_i\subst{t'_1/x_1\ldots t'_n/x_n}} \ t_i} \]
when $x_i$ does not occur rigidly in $A'$,
and this case is provided for by the inductive hypothesis,
or $\top$ otherwise, which we derive using \topGoal.
